# Supplementary material for: On the Impact of Feature Heterophily on Link Prediction with Graph Neural Networks
Source: arXiv:2409.17475 source file (2024-09-26)
Supplement: Supplementary file 1 [file 091appendix-notation.tex]

\newpage
\section{Nomenclature}
\label{app:dfn}

We summarize the main symbols used in this work and their definitions below:

\begin{table}[h!]
     \caption{Major symbols and definitions.} % \reminder{to add more symbols}}
     \label{tab:dfn}
     \resizebox{\textwidth}{!}{
    \begin{tabular}{ lp{11cm}}
         \toprule
         \textbf{Symbols} &  \textbf{Definitions}\\
         \midrule
         $\graph = (\vertexSet, \edgeSet)$ & graph $\graph$ with nodeset $\vertexSet$, edgeset $\edgeSet$ \\
         $\matA$ & $n \times n$ adjacency matrix of $\graph$ \\
         $\matX$ & $n \times F$ node feature matrix of $\graph$ \\
         $\V{x}_v$ & $F$-dimensional feature vector for node $v$ \\
         $\matL$ & unnormalized graph Laplacian matrix \\ 
         \midrule
         $\setY$ & set of class labels\\
         $y_v$ & class label for node $v \in \vertexSet$ \\
         $\vecy$ & $n$-dimensional vector of class labels (for all the nodes)\\
         \midrule
         $\setT = \{(v_1,y_1), (v_2, y_2), ...\}$ & training data for semi-supervised node classification \\
         $N(v)$ & general type of neighbors of node $v$ in graph $\graph$ \\
         $\neighNoSelfLoop(v)$ & general type of neighbors of node $v$ in $\graph$  \textit{without self-loops} (i.e., excluding $v$)  \\
         $N_i(v),\neighNoSelfLoop_i(v)$ & $i$-hop/step neighbors of node $v$ in $\graph$ (at exactly distance $i$) maybe-with/without self-loops, resp.\\
         $\edgeSet_2$ & set of pairs of nodes $(u,v)$ with shortest distance between them being 2 \\
         $d, d_{\mathrm{max}}$ & node degree, and maximum node degree across all nodes $v \in \vertexSet$, resp. \\
         \midrule
         $h$ & edge homophily ratio \\
         $\matH$ & class compatibility matrix \\
        \midrule
         $\V{r}^{(k)}_v$ & node representations learned in GNN model at round / layer $k$ \\
         $K$ & the number of rounds in the neighborhood aggregation stage \\
         $\matW$ & learnable weight matrix for GNN model \\
         $\sigma$ & non-linear activation function \\
         $\Vert$ & vector concatenation operator \\
         \texttt{AGGR} & function that aggregates node feature representations within a neighborhood \\
         \texttt{COMBINE} & function that combines feature representations from different neighborhoods \\
         \bottomrule
    \end{tabular}
    }
    \end{table}
