# Supplementary material for: On the Impact of Feature Heterophily on Link Prediction with Graph Neural Networks
Source: arXiv:2409.17475 source file (2024-09-26)
Supplement: Supplementary file 2 [file 094appendix-tuning.tex]

%\newpage
\vspace{0.3cm}
\section{Experimental Setup \& Hyperparameter Tuning}
\label{app:tuning}

\subsection{Setup} 

\paragraph{\method Implementation} We use $K = 1$ for \method-1 and $K=2$ for \method-2. 
For loss function, we calculate the cross entropy between the predicted 
and the ground-truth labels for nodes within the training set, and add $L_2$ regularization of network parameters $\V{W}_{e}$ and $\V{W}_{c}$. (cf.\ Alg.~\ref{algo:method})

\paragraph{Baseline Implementations} For all baselines besides MLP, we used the official implementation released by the authors on GitHub. 

\begin{itemize}
    \item \textbf{GCN \& GCN-Cheby}~\cite{kipf2016semi}: \url{https://github.com/tkipf/gcn}
    \item \textbf{GraphSAGE}~\cite{hamilton2017inductive}: \url{https://github.com/williamleif/graphsage-simple} (PyTorch implementation)
    \item \textbf{MixHop}~\cite{MixHop}: \url{https://github.com/samihaija/mixhop}
    \item \textbf{GAT}~\cite{velickovic2018graph}: \url{https://github.com/PetarV-/GAT}. (For large datasets, we make use of the sparse version provided by the author.)
\end{itemize}

For MLP, we used our own implementation of MLP with 1-hidden layer, which is equivalent to the case of $K=0$ in Algorithm 1. We use the same loss function as \method for training MLP. 

\paragraph{Hardware Specifications} We run experiments on synthetic benchmarks with an Amazon EC2 instance with instance size as \texttt{p3.2xlarge}, which features an 8-core CPU, 61 GB Memory, and a Tesla V100 GPU with 16 GB GPU Memory. 
For experiments on real benchmarks, we use a workstation with a 12-core AMD Ryzen 9 3900X CPU, 64GB RAM, and a Quadro P6000 GPU with 24 GB GPU Memory.

\subsection{Tuning the GNN Models}

To avoid bias, we tuned the hyperparameters of each method (\method and baseline models) on each benchmark. 
Below we list the hyperparameters tested on each benchmark per model. 
As the hyperparameters defined by each baseline model differ significantly, we list the combinations of non-default command line arguments we tested, without explaining them in detail. % the meaning of each argument. These command line arguments are defined in the implementations of the baseline models and control the hyperparameters of each model; interesting readers can refer to the original implementation for further details. 
We refer the interested reader to the corresponding original implementations for further details on the arguments, including their definitions. 

\paragraph{Synthetic Benchmark Tuning} For each synthetic benchmark, we report the results for different heterophily levels under the same set of hyperparameters for each method, so that we can compare how the same hyperparameters perform across the full spectrum of low-to-high homophily. 
We report the best performance, for the set of hyperparameters which performs the best on the validation set on the majority of the heterophily levels for each method. 

For \texttt{syn-cora}, we test the following command-line arguments for each baseline method: 
\begin{itemize}
    \item \textbf{\method-1 \& \method-2}: 
    \begin{itemize}
        \item Dimension of Feature Embedding $p$: 64
        \item Non-linearity Function $\sigma$: ReLU
        \item Dropout Rate: $a\in \{0, 0.5\}$
    \end{itemize}
    We report the best performance, for $a=0$. 
    \item \textbf{GCN}~\cite{kipf2016semi}: 
    \begin{itemize}
        \item \texttt{\lstinline{hidden1}}: $a\in \{16, 32, 64\}$
        \item \texttt{\lstinline{early_stopping}}: $b\in\{40, 100, 200\}$
        \item \texttt{\lstinline{epochs}}: 2000
    \end{itemize}
    % with $a, b \in \{16, 32, 64\} \times \{40, 100, 200\}$. 
    We report the best performance, for $a=32, b=40$.
    \item \textbf{GCN-Cheby}~\cite{kipf2016semi}: 
    \begin{itemize}
        \item Set 1:
        \begin{itemize}
        \item \texttt{\lstinline{hidden1}}: $a\in\{16, 32, 64\}$
        \item \texttt{\lstinline{dropout}}: 0.6
        \item \texttt{\lstinline{weight_decay}}: $b\in\{\texttt{1e-5, 5e-4}\}$
        \item \texttt{\lstinline{max_degree}}: 2
        \item \texttt{\lstinline{early_stopping}}: 40
        \end{itemize}
        % with $a, b \in \{16, 32, 64\} \times \{\texttt{1e-5, 5e-4}\}$ 
        \item Set 2:
        \begin{itemize}
        \item \texttt{\lstinline{hidden1}}: $a$ $\in \{16, 32, 64\}$
        \item \texttt{\lstinline{dropout}}: 0.5
        \item \texttt{\lstinline{weight_decay}}: \texttt{5e-4}
        \item \texttt{\lstinline{max_degree}}: 3
        \item \texttt{\lstinline{early_stopping}}: 40
    \end{itemize}
    \end{itemize}
    We report the best performance, for Set 1 with $a=64, b=\texttt{5e-4}$.
    \item \textbf{GraphSAGE}~\cite{hamilton2017inductive}: 
    \begin{itemize}
        \item \texttt{\lstinline{hid_units}}: $a\in \{64, 128\}$
        \item \texttt{\lstinline{lr}}: $b\in \{0.1, 0.7\}$
        \item \texttt{\lstinline{epochs}}: 500
    \end{itemize}
    % with $a, b \in \{64, 128\} \times \{0.1, 0.7\}$.
    We report the performance with $a=64, b=0.7$.
    
    \item \textbf{MixHop}~\cite{MixHop}: 
    \begin{itemize}
        \item \texttt{\lstinline{hidden_dims_csv}}: $a \in \{64, 192\}$
        \item \texttt{\lstinline{adj_pows}}: 0, 1, 2
    \end{itemize}
    We report the performance with $a=192$.
    \item \textbf{GAT}~\cite{velickovic2018graph}: 
    \begin{itemize}
        \item \texttt{\lstinline{hid_units}}: $a \in \{8, 16, 32, 64\}$
        \item \texttt{\lstinline{n_heads}}: $b\in\{1, 4, 8\}$ 
    \end{itemize}
    % with $a, b \in \{8, 16, 32, 64\} \times \{1, 4, 8\}$. 
    We report the performance with $a=8, b=8$.
    \item \textbf{MLP}
    \begin{itemize}
        \item Dimension of Feature Embedding $p$: 64
        \item Non-linearity Function $\sigma$: ReLU
        \item Dropout Rate: 0.5
    \end{itemize}
\end{itemize}

For \texttt{syn-products}, we test the following command-line arguments for each baseline method: 
\begin{itemize}
    \item \textbf{\method-1 \& \method-2}: 
    \begin{itemize}
        \item Dimension of Feature Embedding $p$: 64
        \item Non-linearity Function $\sigma$: ReLU
        \item Dropout Rate: $a \in \{0, 0.5\}$
    \end{itemize}
    We report the best performance, for $a=0.5$. 
    \item \textbf{GCN}~\cite{kipf2016semi}: 
    \begin{itemize}
        \item \texttt{\lstinline{hidden1}}: 64
        \item \texttt{\lstinline{early_stopping}}: $a \in \{40, 100, 200\}$
        \item \texttt{\lstinline{epochs}}: 2000
    \end{itemize}
    In addition, we disabled the default feature normalization in the official implementation, as the feature vectors in this benchmark have already been normalized, and we found the default normalization method hurts the performance significantly. We report the best performance, for $a=40$.
    \item \textbf{GCN-Cheby}~\cite{kipf2016semi}: 
    \begin{itemize}
        \item \texttt{\lstinline{hidden1}}: 64
        \item \texttt{\lstinline{max_degree}}: 2
        \item \texttt{\lstinline{early_stopping}}: 40
        \item \texttt{\lstinline{epochs}}: 2000
        % \item \texttt{\lstinline{weight_decay}}: $a \in \{\texttt{1e-5, 5e-4}\}$
    \end{itemize}
    We also disabled the default feature normalization in the official implementation for this baseline. %We report the best performance, for %$a=40$.
    \item \textbf{GraphSAGE}~\cite{hamilton2017inductive}: 
    \begin{itemize}
        \item \texttt{\lstinline{hid_units}}: $a \in \{64, 128\}$
        \item \texttt{\lstinline{lr}}: $b \in \{0.1, 0.7\}$
        \item \texttt{\lstinline{epochs}}: 500
    \end{itemize}
    % with $a, b \in \{64, 128\} \times \{0.1, 0.7\}$.
    We report the performance with $a=128, b=0.1$.
    \item \textbf{MixHop}~\cite{MixHop}: 
    \begin{itemize}
        \item \texttt{\lstinline{hidden_dims_csv}}: $a \in \{64, 192\}$
        \item \texttt{\lstinline{adj_pows}}: 0, 1, 2
    \end{itemize}
    We report the performance with $a=192$.
    \item \textbf{GAT}~\cite{velickovic2018graph}: 
    \begin{itemize}
        \item \texttt{\lstinline{hid_units}}: $8$
    \end{itemize}
    We also disabled the default feature normalization in the official implementation for this baseline.
    \item \textbf{MLP}
    \begin{itemize}
        \item Dimension of Feature Embedding $p$: 64
        \item Non-linearity Function $\sigma$: ReLU
        \item Dropout Rate: 0.5
    \end{itemize}
\end{itemize}

\paragraph{Real Benchmark (except {Cora-Full}) Tuning} For each real benchmark in Table~\ref{tab:5-real-results} (except \textbf{Cora-Full}),  
we perform hyperparameter tuning (see values below) and report the best performance of each method 
on the validation set. So, for each method, its performance on different benchmarks can be reported from different hyperparameters. We test the following command-line arguments for each baseline method: 
\begin{itemize}
    \item \textbf{\method-1 \& \method-2}: %
    \begin{itemize}
        \item Dimension of Feature Embedding $p$: 64
        \item Non-linearity Function $\sigma$: \{\texttt{ReLU, None}\}
        \item Dropout Rate: $\{0, 0.5\}$
        \item L2 Regularization Weight: \{\texttt{1e-5, 5e-4}\}
    \end{itemize}
    \item \textbf{GCN}~\cite{kipf2016semi}: % 
    \begin{itemize}
        \item \texttt{\lstinline{hidden1}}: 64
        \item \texttt{\lstinline{early_stopping}}: $\{40, 100, 200\}$
        \item \texttt{\lstinline{epochs}}: 2000
    \end{itemize}
    \item \textbf{GCN-Cheby}~\cite{kipf2016semi}: % 
    \begin{itemize}
        % \item Set 1:
        % \begin{itemize}
        \item \texttt{\lstinline{hidden1}}: 64
        \item \texttt{\lstinline{weight_decay}}: $\{\texttt{1e-5, 5e-4}\}$
        \item \texttt{\lstinline{max_degree}}: 2
        \item \texttt{\lstinline{early_stopping}}: $\{40, 100, 200\}$
        \item \texttt{\lstinline{epochs}}: 2000
    \end{itemize}
    \item \textbf{GraphSAGE}~\cite{hamilton2017inductive}: % 
    \begin{itemize}
        \item \texttt{\lstinline{hid_units}}: 64
        \item \texttt{\lstinline{lr}}: $\{0.1, 0.7\}$
        \item \texttt{\lstinline{epochs}}: 500
    \end{itemize}
    \item \textbf{MixHop}~\cite{MixHop}: %
    \begin{itemize}
        \item \texttt{\lstinline{hidden_dims_csv}}: $\{64, 192\}$
        \item \texttt{\lstinline{adj_pows}}: 0, 1, 2
    \end{itemize}
    \item \textbf{GAT}~\cite{velickovic2018graph}: 
    \begin{itemize}
        \item \texttt{\lstinline{hid_units}}: $8$
    \end{itemize}
    \item \textbf{MLP}
    \begin{itemize}
        \item Dimension of Feature Embedding $p$: 64
        \item Non-linearity Function $\sigma$: $\{\texttt{ReLU, None}\}$
        \item Dropout Rate: $\{0, 0.5\}$
    \end{itemize}
    % with $a, b \in \{\texttt{ReLU, None}\} \times \{0, 0.5\}$.
\end{itemize}

For \textbf{GCN+JK}, \textbf{GCN-Cheby+JK} and \textbf{GraphSAGE+JK}, %
we enhanced the corresponding base model with jumping knowledge (JK) connections using JK-Concat~\cite{XuLTSKJ18-jkn} \emph{without} changing the number of layers or other hyperparameters for the base method.

\paragraph{Cora Full Benchmark Tuning}
The number of class labels in Cora-Full are many more compared to the other benchmarks (Table~\ref{tab:5-real-results}), which 
leads to a significant increase in the size of training parameters for each model. Therefore, we need to re-tune the hyperparameters, especially the regularization weights and learning rates, in order to get reasonable performance. We test the following command-line arguments for each baseline method: 
\begin{itemize}
    \item \textbf{\method-1 \& \method-2}: %
    \begin{itemize}
        \item Dimension of Feature Embedding $p$: 64
        \item Non-linearity Function $\sigma$: $\{\texttt{ReLU, None}\}$
        \item Dropout Rate: $\{0, 0.5\}$
        \item L2 Regularization Weight: $\{\texttt{1e-5, 1e-6}\}$
        % \item Learning Rate: $c \in \{ 0.01, 0.05\}$
    \end{itemize}
    % with $a, b, c \in \{\texttt{ReLU, None}\} \times \{\texttt{1e-5, 1e-6}\} \times \{ 0.01, 0.05\}$
    \item \textbf{GCN}~\cite{kipf2016semi}: %
    \begin{itemize}
        \item \texttt{\lstinline{hidden1}}: 64
        \item \texttt{\lstinline{early_stopping}}: $\{40, 100, 200\}$
        \item \texttt{\lstinline{weight_decay}:} $\{\texttt{5e-5, 1e-5, 1e-6}\}$
        \item \texttt{\lstinline{epochs}}: 2000
    \end{itemize}
    \item \textbf{GCN-Cheby}~\cite{kipf2016semi}: %
    \begin{itemize}
        \item \texttt{\lstinline{hidden1}}: 64
        \item \texttt{\lstinline{weight_decay}}: $\{\texttt{5e-5, 1e-5, 1e-6}\}$
        \item \texttt{\lstinline{max_degree}}: 2
        \item \texttt{\lstinline{early_stopping}}: $\{40, 100, 200\}$
        \item \texttt{\lstinline{epochs}}: 2000
    \end{itemize}
    \item \textbf{GraphSAGE}~\cite{hamilton2017inductive}: %
    \begin{itemize}
        \item \texttt{\lstinline{hid_units}}: 64
        \item \texttt{\lstinline{lr}}: 0.7
        \item \texttt{\lstinline{epochs}}: 2000
    \end{itemize}
    % with $a, b \in \{64, 128\} \times \{0.1, 0.7\}$.
    \item \textbf{MixHop}~\cite{MixHop}: %
    \begin{itemize}
        \item \texttt{\lstinline{adj_pows}}: 0, 1, 2
        \item \texttt{\lstinline{hidden_dims_csv}}: $\{64, 192\}$
        \item \texttt{\lstinline{l2reg}}: $\{\texttt{5e-4, 5e-5}\}$
    \end{itemize}
    \item \textbf{GAT}~\cite{velickovic2018graph}: 
    \begin{itemize}
        \item \texttt{\lstinline{hid_units}}: $8$
        \item \texttt{\lstinline{l2_coef}}: $\{\texttt{5e-4, 5e-5, 1e-5}\}$
    \end{itemize}
    \item \textbf{MLP}
    \begin{itemize}
        \item Dimension of Feature Embedding $p$: 64
        \item Non-linearity Function $\sigma$: $\{\texttt{ReLU, None}\}$
        \item Dropout Rate: $\{0, 0.5\}$
        \item L2 Regularization Weight: \texttt{1e-5}
        \item Learning Rate: 0.05
    \end{itemize}
\end{itemize}

For \textbf{GCN+JK}, \textbf{GCN-Cheby+JK} and \textbf{GraphSAGE+JK}, 
we enhanced the corresponding base model with jumping knowledge (JK) connections using JK-Concat~\cite{XuLTSKJ18-jkn} \emph{without} changing the number of layers or other hyperparameters for the base method.
