# Supplementary material for: On the Impact of Feature Heterophily on Link Prediction with Graph Neural Networks
Source: arXiv:2409.17475 source file (2024-09-26)
Supplement: Supplementary file 3 [file 095-appendix-synthetic.tex]

\newpage
\section{Synthetic Datasets: Details}
\label{app:synthetic}

\subsection{Data Generation Process \& Setup}

\paragraph{Synthetic graph generation} We generate synthetic graphs with various heterophily levels by adopting an approach similar to \cite{MixHop, karimi2017visibility17}. In general, the synthetic graphs are generated by a modified preferential attachment process \cite{Barabasi:1999}: The number of class labels $|\setY|$ in the synthetic graph is prescribed. Then, starting from a small initial graph, new nodes are added into the graph one by one, until the number of nodes $|\vertexSet|$ has reached the preset level. The probability $p_{uv}$ for a newly added node $u$ in class $i$ to connect with an existing node $v$ in class $j$ is proportional to both the class compatibility $H_{ij}$ between class $i$ and $j$, and the degree $d_v$ of the existing node $v$. As a result, the degree distribution for the generated graphs follow a power law, and the heterophily can be controlled by class compatibility matrix $\matH$. 
Table \ref{tab:5-synthetic-data} shows an overview of these synthetic benchmarks, and more detailed statistics 
can be found in Table~\ref{tab:A-synthetic-stats}. 

\paragraph{Node features \& classes} Nodes are assigned randomly to each class during the graph generation. Then, in each synthetic graph, the feature vectors of nodes in each class are generated by sampling feature vectors of nodes from the corresponding class in a real benchmark (e.g., Cora~\cite{sen2008collective, yang2016revisiting}  or \texttt{ogbn-products}~\cite{hu2020ogb}): 
We first establish a class mapping $\psi: \setY_s \rightarrow \setY_b$ between classes in the synthetic graph $\setY_s$ to classes in an existing benchmark $\setY_b$. The only requirement is that the class size in the existing benchmark is larger than that of the synthetic graph so that an injection between nodes from both classes can be established, and the feature vectors for the synthetic graph can be sampled accordingly.   
For \texttt{syn-products}, we further restrict the feature sampling to ensure that nodes in the training, validation and test splits are only mapped to nodes in the corresponding splits in the benchmark. This process respects the data splits used in \texttt{ogbn-products}, which are more realistic and challenging than random splits~\cite{hu2020ogb}. For simplicity, in our synthetic benchmarks, all the classes (5 for \texttt{syn-cora} and 10 for \texttt{syn-products} -- Table~\ref{tab:A-synthetic-stats}) are of the same size.

\begin{table}[h]
% \begin{wraptable}{r}{0.4\textwidth}
	\centering
	% \vspace{-0.3cm}
	\caption{Statistics for Synthetic Datasets} % \reminder{fill out and add other important symbols}} 
	\label{tab:A-synthetic-stats}
	% \resizebox{\columnwidth}{!}{
	{\footnotesize
	\begin{tabular}{lcc}
		\toprule 
		% \specialrule{.1em}{.05em}{.05em} 
		\textbf{Benchmark Name} & \texttt{syn-cora} & \texttt{syn-products} \\
		\midrule
		\textbf{\# Nodes} & 1490 & 10000 \\
		\textbf{\# Edges} & 2965 to 2968  & 59640 to 59648 \\
		\textbf{\# Classes} & 5 & 10 \\
		% \textbf{$\V{H}$ Control} & Scalar & Scalar \\
		\textbf{Features} 
		    & \texttt{cora}~\cite{sen2008collective, yang2016revisiting} 
		    & \texttt{ogbn-products}~\cite{hu2020ogb} \\
		\textbf{Homophily $h$} & [0, 0.1, \ldots, 1] & [0, 0.1, \ldots, 1] \\
		\textbf{Degree Range} & 1 to 94 & 1 to 336 \\
		\textbf{Average Degree} & 3.98 & 11.93 \\
		\bottomrule
	\end{tabular}
	}
\end{table}

\paragraph{Experimental setup} For each heterophily ratio $h$ of each benchmark, we independently generate 3 different graphs. For \texttt{syn-cora} and \texttt{syn-products}, we randomly partition 25\% of nodes into training set, 25\% into validation and 50\% into test set.  
All methods share the same training, partition and test splits, and the average and standard derivation of the performance values under the 3 generated graphs are reported as the performance under each heterophily level of each benchmark.

\subsection{Detailed Results on Synthetic Benchmarks}
\label{app:synthetic-results}

Tables~\ref{tab:app-syn-cora-results} and \ref{tab:app-syn-products-results} give the results on \texttt{syn-cora} and \texttt{syn-products} shown in Figure~\ref{fig:5-syn-results} of the main paper (\S~\ref{sec:eval-synthetic}).
Table~\ref{tab:design-ablations} provides the detailed results of the ablation studies that we designed in order to investigate the significance of our design choices, and complements Fig.~\ref{fig:design-ablations} in \S~\ref{sec:eval-synthetic}.

\begin{table}[t]
	\centering
	\caption{\texttt{syn-cora} (Fig.~\ref{fig:syn-cora}): Mean accuracy and standard deviation per method and synthetic dataset (with different homophily ratio $h$). Best method highlighted in gray.}  
	\label{tab:app-syn-cora-results}
    \resizebox{.7\textwidth}{!}{
	\begin{tabular}{lcccccc}
		\toprule 
		\textbf{h} & \textbf{0.00} & \textbf{0.10} & \textbf{0.20} & \textbf{0.30} & \textbf{0.40} & \textbf{0.50}  \\ \midrule %\vspace{0.05cm}
		\textbf{\method-1} & $77.40{\scriptstyle\pm0.89}$ & $76.82{\scriptstyle\pm1.30}$ & $73.38{\scriptstyle\pm0.95}$ & \cellcolor{gray!15}$75.26{\scriptstyle\pm0.56}$ & $75.66{\scriptstyle\pm2.19}$ & \cellcolor{gray!15}$80.22{\scriptstyle\pm1.35}$ \\ 
		
		% HistFNN --network_setup M64-R-G-V-G-V-MO --hist_nhood 0 1 2
		\textbf{\method-2} & \cellcolor{gray!15}$77.85{\scriptstyle\pm1.63}$ & \cellcolor{gray!15}$76.87{\scriptstyle\pm0.43}$ & \cellcolor{gray!15}$74.27{\scriptstyle\pm1.30}$ & $74.41{\scriptstyle\pm0.43}$ & \cellcolor{gray!15}$76.33{\scriptstyle\pm1.35}$ & $79.60{\scriptstyle\pm0.48}$ \\
        
		\textbf{GraphSAGE} & $75.97{\scriptstyle \pm1.94}$ & $72.89{\scriptstyle \pm2.42}$ & $70.56{\scriptstyle \pm1.42}$ & $71.81{\scriptstyle \pm0.67}$ & $72.04{\scriptstyle \pm1.68}$ & $76.55{\scriptstyle \pm0.81}$ \\
		\textbf{GCN-Cheby} & $74.23{\scriptstyle \pm0.54}$ & $68.10{\scriptstyle \pm1.75}$ & $64.70{\scriptstyle \pm1.17}$ & $66.71{\scriptstyle \pm1.63}$ & $68.14{\scriptstyle \pm1.56}$ & $73.33{\scriptstyle \pm2.05}$ \\
		\textbf{MixHop} & $62.64{\scriptstyle\pm1.16}$ & $58.93{\scriptstyle\pm2.84}$ & $60.89{\scriptstyle\pm1.20}$ & $65.73{\scriptstyle\pm0.41}$ & $67.87{\scriptstyle\pm4.01}$ & $70.11{\scriptstyle\pm0.34}$ \\
		\midrule
		% HistFNN --network_setup M64-R-D-MO
		% --model gcn --hidden1 32 --early_stopping 40
		\textbf{GCN} & $33.65{\scriptstyle \pm1.68}$ & $37.14{\scriptstyle \pm4.60}$ & $42.82{\scriptstyle \pm1.89}$ & $51.10{\scriptstyle \pm0.77}$ & $56.91{\scriptstyle \pm2.56}$ & $66.22{\scriptstyle \pm1.04}$ \\
		% --model gcn_cheby --hidden1 64 --dropout 0.6 --weight_decay 5e-4 --max_degree 2 --early_stopping 40
		% --adj_pows=0,1,2 --retrain
		% --hid_units 8 --n_heads 8 1
		\textbf{GAT} & $30.16{\scriptstyle \pm1.32}$ & $33.11{\scriptstyle \pm1.20}$ & $39.11{\scriptstyle \pm0.28}$ & $48.81{\scriptstyle \pm1.57}$ & $55.35{\scriptstyle \pm2.35}$ & $64.52{\scriptstyle \pm0.47}$ \\ 
		\midrule
		\textbf{MLP} & $72.75{\scriptstyle \pm1.51}$ & $74.85{\scriptstyle \pm0.76}$ & $74.05{\scriptstyle \pm0.69}$ & $73.78{\scriptstyle \pm1.14}$ & $73.33{\scriptstyle \pm0.34}$ & $74.81{\scriptstyle \pm1.90}$ \\
		\bottomrule
        \toprule
        \textbf{h} & \textbf{0.60} & \textbf{0.70} & \textbf{0.80} & \textbf{0.90} & \textbf{1.00}\\
        \midrule
        \textbf{\method-1} & $83.62{\scriptstyle\pm0.82}$ & $88.14{\scriptstyle\pm0.31}$ & $91.63{\scriptstyle\pm0.77}$ & $95.53{\scriptstyle\pm0.61}$ & $99.06{\scriptstyle\pm0.27}$ \\
        
        \textbf{\method-2} & \cellcolor{gray!15}$84.43{\scriptstyle\pm1.89}$ & \cellcolor{gray!15}$88.28{\scriptstyle\pm0.66}$ & \cellcolor{gray!15}$92.39{\scriptstyle\pm1.34}$ & \cellcolor{gray!15}$95.97{\scriptstyle\pm0.59}$ & \cellcolor{gray!15}$100.00{\scriptstyle\pm0.00}$ \\

        \textbf{GraphSAGE} & $81.25{\scriptstyle \pm1.04}$ & $85.06{\scriptstyle \pm0.51}$ & $90.78{\scriptstyle \pm1.02}$ & $95.08{\scriptstyle \pm1.16}$  & $99.87{\scriptstyle \pm0.00}$ \\
        \textbf{GCN-Cheby} & $78.88{\scriptstyle \pm0.21}$ & $84.92{\scriptstyle \pm1.03}$ & $90.92{\scriptstyle \pm1.62}$ & $95.97{\scriptstyle \pm1.07}$ & \cellcolor{gray!15} ${100.00{\scriptstyle \pm0.00}}$ \\
        \textbf{MixHop} & $79.78{\scriptstyle\pm1.92}$ & $84.43{\scriptstyle\pm0.94}$ & $91.90{\scriptstyle\pm2.02}$ & $96.82{\scriptstyle\pm0.08}$ & $100.00{\scriptstyle\pm0.00}$ \\
        \midrule
        \textbf{GCN} & $77.32{\scriptstyle \pm1.17}$ & $84.52{\scriptstyle \pm0.54}$ & $91.23{\scriptstyle \pm1.29}$ & $96.11{\scriptstyle \pm0.82}$ & \cellcolor{gray!15} ${100.00{\scriptstyle \pm0.00}}$ \\
  		\textbf{GAT} & $76.29{\scriptstyle \pm1.83}$ & $84.03{\scriptstyle \pm0.97}$ & $90.92{\scriptstyle \pm1.51}$ & $95.88{\scriptstyle \pm0.21}$ & \cellcolor{gray!15} ${100.00{\scriptstyle \pm0.00}}$ \\
  		\midrule
        \textbf{MLP} & $73.42{\scriptstyle \pm1.07}$ & $71.72{\scriptstyle \pm0.62}$ & $72.26{\scriptstyle \pm1.53}$ & $72.53{\scriptstyle \pm2.77}$ & $73.65{\scriptstyle \pm0.41}$ \\
        \bottomrule
	\end{tabular}
}
\end{table}

\begin{table}[t]
	\caption{\texttt{syn-products} (Fig.~\ref{fig:syn-products}): Mean accuracy and standard deviation per method and synthetic dataset (with different homophily ratio $h$). Best method highlighted in gray.} 
	\label{tab:app-syn-products-results}  %\cellcolor{gray!15}
	\centering
    \resizebox{.7\textwidth}{!}{
	\begin{tabular}{lcccccc}
		\toprule 	
		\textbf{h} & \textbf{0.00} & \textbf{0.10} & \textbf{0.20} & \textbf{0.30} & \textbf{0.40} & \textbf{0.50}  \\ \midrule %\vspace{0.05cm}
		% HistFNN --network_setup M64-R-T1-G-V-C1-D0.5-MO --hist_nhood 1 2 --no_feature_normalize
		\textbf{\method-1}  & $82.06{\scriptstyle \pm0.24}$ & $78.39{\scriptstyle \pm1.56}$ & $79.37{\scriptstyle \pm0.21}$ & $81.10{\scriptstyle \pm0.22}$ & $84.25{\scriptstyle \pm1.08}$ & $88.15{\scriptstyle \pm0.28}$ \\
		% HistFNN --network_setup M64-R-T1-G-V-T2-G-V-C1-C2-D0.5-MO --hist_nhood 1 2 --no_feature_normalize
		\textbf{\method-2} & $83.37{\scriptstyle \pm0.38}$ & \cellcolor{gray!15} $80.03{\scriptstyle \pm0.84}$ & \cellcolor{gray!15} $81.09{\scriptstyle \pm0.41}$ & \cellcolor{gray!15} $82.79{\scriptstyle \pm0.49}$ & \cellcolor{gray!15} $86.73{\scriptstyle \pm0.66}$ & \cellcolor{gray!15} $90.75{\scriptstyle \pm0.43}$ \\
		\textbf{GraphSAGE} & $77.66{\scriptstyle \pm0.72}$ & $74.04{\scriptstyle \pm1.07}$ & $75.29{\scriptstyle \pm0.82}$ & $76.39{\scriptstyle \pm0.24}$ & $80.49{\scriptstyle \pm0.96}$ & $84.51{\scriptstyle \pm0.51}$\\
		% --model gcn_cheby --hidden1 64 --max_degree 2 --early_stopping 40 --no_feature_normalize
		\textbf{GCN-Cheby} & \cellcolor{gray!15} $84.35{\scriptstyle \pm0.62}$ & $76.95{\scriptstyle \pm0.30}$ & $77.07{\scriptstyle \pm0.49}$ & $78.43{\scriptstyle \pm0.73}$ & $85.09{\scriptstyle \pm0.29}$ & $89.66{\scriptstyle \pm0.53}$ \\
		% --adj_pows=0,1,2 --retrain
		\textbf{MixHop} & $15.39{\scriptstyle\pm1.38}$ & $11.91{\scriptstyle\pm1.17}$ & $14.03{\scriptstyle\pm1.70}$ & $14.92{\scriptstyle\pm0.56}$ & $17.04{\scriptstyle\pm0.40}$ & $18.90{\scriptstyle\pm1.49}$ \\
		\midrule
		% --model gcn --hidden1 64 --early_stopping 40 --no_feature_normalize
		\textbf{GCN} & $56.44{\scriptstyle \pm0.59}$ & $51.51{\scriptstyle \pm0.56}$ & $54.97{\scriptstyle \pm0.66}$ & $64.90{\scriptstyle \pm0.90}$ & $76.25{\scriptstyle \pm0.04}$ & $86.43{\scriptstyle \pm0.58}$ \\
		% --hid_units 128 --lr 0.1 --epochs 500
		\textbf{GAT} & $27.39{\scriptstyle\pm2.47}$ & $21.49{\scriptstyle\pm2.25}$ & $37.27{\scriptstyle\pm3.99}$ & $44.46{\scriptstyle\pm0.68}$ & $51.86{\scriptstyle\pm8.52}$ & $69.42{\scriptstyle\pm5.30}$ \\
		\midrule
		% HistFNN --network_setup F64-R-D-FO --no_feature_normalize
		\textbf{MLP} & $68.63{\scriptstyle \pm0.58}$ & $68.20{\scriptstyle \pm1.20}$ & $68.85{\scriptstyle \pm0.73}$ & $68.65{\scriptstyle \pm0.18}$ & $68.37{\scriptstyle \pm0.85}$ & $68.70{\scriptstyle \pm0.61}$ \\
		\bottomrule
        \toprule
        \textbf{h} & \textbf{0.60} & \textbf{0.70} & \textbf{0.80} & \textbf{0.90} & \textbf{1.00}\\
        \midrule
        \textbf{\method-1} & $92.39{\scriptstyle \pm0.06}$ & $95.69{\scriptstyle \pm0.19}$ & $98.09{\scriptstyle \pm0.23}$ & $99.63{\scriptstyle \pm0.13}$ & $99.93{\scriptstyle \pm0.01}$ \\
        \textbf{\method-2} & $94.81{\scriptstyle \pm0.27}$ & $97.67{\scriptstyle \pm0.18}$ & $99.13{\scriptstyle \pm0.05}$ & $99.89{\scriptstyle \pm0.08}$ & $99.99{\scriptstyle \pm0.01}$ \\
        \textbf{GraphSAGE} & $89.51{\scriptstyle \pm0.29}$ & $93.61{\scriptstyle \pm0.52}$ & $96.66{\scriptstyle \pm0.19}$ & $98.78{\scriptstyle \pm0.11}$ & $99.63{\scriptstyle \pm0.08}$ \\
        \textbf{GCN-Cheby} & \cellcolor{gray!15} $94.99{\scriptstyle \pm0.34}$ & \cellcolor{gray!15} $98.26{\scriptstyle \pm0.11}$ & \cellcolor{gray!15} $99.58{\scriptstyle \pm0.11}$ & \cellcolor{gray!15} $99.93{\scriptstyle \pm0.06}$ & \cellcolor{gray!15} $100.00{\scriptstyle \pm0.00}$ \\
        \textbf{MixHop} & $19.47{\scriptstyle\pm5.21}$ & $21.15{\scriptstyle\pm2.28}$ & $24.16{\scriptstyle\pm3.19}$ & $23.21{\scriptstyle\pm5.30}$ & $25.09{\scriptstyle\pm5.08}$ \\
        \midrule
        \textbf{GCN} & $93.35{\scriptstyle \pm0.28}$ & $97.61{\scriptstyle \pm0.24}$ & $99.33{\scriptstyle \pm0.08}$ & \cellcolor{gray!15}$99.93{\scriptstyle \pm0.01}$  & $99.99{\scriptstyle \pm0.01}$ \\
		\textbf{GAT} & $85.36{\scriptstyle\pm3.67}$ & $93.52{\scriptstyle\pm1.93}$ & $98.84{\scriptstyle\pm0.12}$ & $99.87{\scriptstyle\pm0.06}$ & $99.98{\scriptstyle\pm0.02}$ \\ 
		\midrule
        \textbf{MLP} & $68.21{\scriptstyle \pm0.93}$ & $68.72{\scriptstyle \pm1.11}$ & $68.10{\scriptstyle \pm0.54}$ & $68.36{\scriptstyle \pm1.42}$ & $69.08{\scriptstyle \pm1.03}$ \\
        \bottomrule
	\end{tabular}
}
\end{table}

\begin{table}[t]
	\caption{Ablation studies of \method to show the significance of designs D1-D3 (Fig.~\ref{fig:design-ablations}(a)-(c)): Mean accuracy and standard deviation per method on the \texttt{syn-products} networks.} 
	\label{tab:design-ablations}
	\centering
    \resizebox{.91\textwidth}{!}{
	\begin{tabular}{l@{\hskip 0.8cm}lcccccc}
		\toprule 
		\textbf{Design} & \textbf{h} & \textbf{0.00} & \textbf{0.10} & \textbf{0.20} & \textbf{0.30} & \textbf{0.40} & \textbf{0.50}  \\ 		
		\midrule %\vspace{0.05cm}
		% HistFNN --network_setup M64-R-T1-G-V-C1-D0.5-MO --hist_nhood 1 2 --no_feature_normalize
		D1-D3 & \textbf{[S0 / K2] \method-1}  & $82.06{\scriptstyle \pm0.24}$ & $78.39{\scriptstyle \pm1.56}$ & $79.37{\scriptstyle \pm0.21}$ & $81.10{\scriptstyle \pm0.22}$ & $84.25{\scriptstyle \pm1.08}$ & $88.15{\scriptstyle \pm0.28}$ \\
		% HistFNN --network_setup M64-R-T1-G-V-T2-G-V-C1-C2-D0.5-MO --hist_nhood 1 2 --no_feature_normalize
		D3 & \textbf{\method-2} & $83.37{\scriptstyle \pm0.38}$ & $80.03{\scriptstyle \pm0.84}$ & $81.09{\scriptstyle \pm0.41}$ & $82.79{\scriptstyle \pm0.49}$ & $86.73{\scriptstyle \pm0.66}$ & $90.75{\scriptstyle \pm0.43}$ \\
		\midrule
		%% 1 Avg-1 (GCN Style, 1+2-hop)
		D1 & \textbf{[NS0] $\mathbf{N_1 + N_2}$} & $52.72{\scriptstyle \pm0.13}$ & $41.65{\scriptstyle \pm0.18}$ & $46.11{\scriptstyle \pm0.86}$ & $58.16{\scriptstyle \pm0.79}$ & $71.10{\scriptstyle \pm0.54}$ & $82.19{\scriptstyle \pm0.40}$ \\
		%% 2 Avg-1 (GCN Style, 1-hop)
		D1 & \textbf{[NS1] Only $\mathbf{N_1}$} & $40.35{\scriptstyle \pm0.58}$ & $35.17{\scriptstyle \pm0.92}$ & $40.35{\scriptstyle \pm0.92}$ & $52.45{\scriptstyle \pm0.85}$ & $65.62{\scriptstyle \pm0.56}$ & $76.05{\scriptstyle \pm0.38}$ \\
	    %% 3 Avg-1 (0+1-hop)
		D1, D2 & \textbf{[S1 / N2] w/o $\neighNoSelfLoop_2$} & $79.65{\scriptstyle \pm0.27}$ & $76.08{\scriptstyle \pm0.76}$ & $76.46{\scriptstyle \pm0.21}$ & $77.29{\scriptstyle \pm0.46}$ & $79.81{\scriptstyle \pm0.88}$ & $83.56{\scriptstyle \pm0.22}$ \\
		%% 4 Avg-1 (0+2-hop)
		D2 & \textbf{[N1] w/o $\neighNoSelfLoop_1$} & $72.27{\scriptstyle \pm0.55}$ & $73.05{\scriptstyle \pm1.23}$ & $75.81{\scriptstyle \pm0.67}$ & $76.83{\scriptstyle \pm0.72}$ & $80.49{\scriptstyle \pm0.72}$ & $82.91{\scriptstyle \pm0.44}$ \\		
	    %% 5 Avg-1 (1+2-hop)
	    D2 & \textbf{[N0] w/o 0-hop neighb. (ego)} & $63.55{\scriptstyle \pm0.46}$ & $46.73{\scriptstyle \pm0.42}$ & $42.29{\scriptstyle \pm0.55}$ & $48.20{\scriptstyle \pm0.59}$ & $61.22{\scriptstyle \pm0.35}$ & $75.15{\scriptstyle \pm0.27}$ \\
		% HistFNN --network_setup M64-R-T1-G-V-T2-G-V-C2-D0.5-MO --hist_nhood 1 2 --no_feature_normalize %% 13 Avg-2 (1+2-iter)
	    D3 &  \textbf{[K0] No Round-0} & $75.63{\scriptstyle \pm0.19}$ & $61.99{\scriptstyle \pm0.57}$ & $56.36{\scriptstyle \pm0.56}$ & $61.27{\scriptstyle \pm0.71}$ & $73.33{\scriptstyle \pm0.88}$ & $84.51{\scriptstyle \pm0.50}$ \\
	    % HistFNN --network_setup M64-R-T1-G-V-T2-G-V-C1-D0.5-MO --hist_nhood 1 2 --no_feature_normalize %% 12 Avg-2 (0+2-iter)
	    D3 & \textbf{[K1] No Round-1} & $75.75{\scriptstyle \pm0.90}$ & $75.65{\scriptstyle \pm0.73}$ & $79.25{\scriptstyle \pm0.18}$ & $81.19{\scriptstyle \pm0.33}$ & $84.64{\scriptstyle \pm0.35}$ & $88.46{\scriptstyle \pm0.60}$ \\
	    % HistFNN --network_setup M64-R-T1-G-V-T2-G-V-D0.5-MO --hist_nhood 1 2 --no_feature_normalize %% 14 Avg-2 (2-iter only)
	    D3 & \textbf{[R2] Only Round-2} & $73.11{\scriptstyle \pm1.01}$ & $62.47{\scriptstyle \pm1.35}$ & $59.99{\scriptstyle \pm0.43}$ & $64.37{\scriptstyle \pm1.14}$ & $75.43{\scriptstyle \pm0.70}$ & $86.02{\scriptstyle \pm0.79}$ \\
	    % HistFNN --network_setup M64-R-T1-G-V-M64-R-T2-G-V-M64-R-C2-C1-D0.5-MO --hist_nhood 0 1 2 --no_feature_normalize
	    \midrule
	    \S~\ref{app:qualitative-comp} & \textbf{Non-linear \method-2 (\S~\ref{app:qualitative-comp})} & $82.23{\scriptstyle \pm0.25}$ & $78.78{\scriptstyle \pm1.04}$ & $80.47{\scriptstyle \pm0.15}$ & $82.08{\scriptstyle \pm0.10}$ & $85.89{\scriptstyle \pm0.53}$ & $89.78{\scriptstyle \pm0.11}$ \\

		\bottomrule \\
        \toprule
        \textbf{Design} & \textbf{h} & \textbf{0.60} & \textbf{0.70} & \textbf{0.80} & \textbf{0.90} & \textbf{0.99} & \textbf{1.00}\\
        \midrule
        D1, D3 & \textbf{[S0 / K2] \method-1} & $92.39{\scriptstyle \pm0.06}$ & $95.69{\scriptstyle \pm0.19}$ & $98.09{\scriptstyle \pm0.23}$ & $99.63{\scriptstyle \pm0.13}$ & $99.88{\scriptstyle \pm0.06}$ & $99.93{\scriptstyle \pm0.01}$ \\
        D3 & \textbf{\method-2} & $94.81{\scriptstyle \pm0.27}$ & $97.67{\scriptstyle \pm0.18}$ & $99.13{\scriptstyle \pm0.05}$ & $99.89{\scriptstyle \pm0.08}$ & $99.98{\scriptstyle \pm0.00}$ & $99.99{\scriptstyle \pm0.01}$ \\
        \midrule
        D1 & \textbf{[NS0] $\mathbf{N_1 + N_2}$} & $90.39{\scriptstyle \pm0.54}$ & $95.25{\scriptstyle \pm0.06}$ & $98.27{\scriptstyle \pm0.13}$ & $99.69{\scriptstyle \pm0.03}$ & $99.98{\scriptstyle \pm0.02}$ & $100.00{\scriptstyle \pm0.00}$ \\
        D1 & \textbf{[NS1] Only $\mathbf{N_1}$} & $84.41{\scriptstyle \pm0.44}$ & $90.15{\scriptstyle \pm0.27}$ & $95.21{\scriptstyle \pm0.34}$ & $97.71{\scriptstyle \pm0.06}$ & $99.56{\scriptstyle \pm0.11}$ & $99.49{\scriptstyle \pm0.11}$ \\
        D1, D2 & \textbf{[S1 / N2] w/o $\neighNoSelfLoop_2$} & $87.39{\scriptstyle \pm0.33}$ & $91.08{\scriptstyle \pm0.50}$ & $94.36{\scriptstyle \pm0.32}$ & $97.01{\scriptstyle \pm0.40}$ & $98.79{\scriptstyle \pm0.23}$ & $98.71{\scriptstyle \pm0.15}$ \\
	    D2 & \textbf{[N1] w/o $\neighNoSelfLoop_1$} & $87.24{\scriptstyle \pm0.21}$ & $92.55{\scriptstyle \pm0.50}$ & $95.64{\scriptstyle \pm0.19}$ & $98.71{\scriptstyle \pm0.13}$ & $99.73{\scriptstyle \pm0.12}$ & $99.83{\scriptstyle \pm0.06}$ \\
        D2 & \textbf{[N0] w/o 0-hop neighb. (ego)} & $86.08{\scriptstyle \pm0.58}$ & $93.03{\scriptstyle \pm0.29}$ & $97.45{\scriptstyle \pm0.09}$ & $99.45{\scriptstyle \pm0.06}$ & $99.98{\scriptstyle \pm0.02}$ & $99.98{\scriptstyle \pm0.03}$ \\
        D3 & \textbf{[K0] No Round-0} & $92.42{\scriptstyle \pm0.13}$ & $96.81{\scriptstyle \pm0.11}$ & $99.09{\scriptstyle \pm0.27}$ & $99.89{\scriptstyle \pm0.01}$ & $100.00{\scriptstyle \pm0.00}$ & $100.00{\scriptstyle \pm0.00}$ \\
        D3 & \textbf{[K1] No Round-1} & $93.05{\scriptstyle \pm0.23}$ & $97.17{\scriptstyle \pm0.36}$ & $99.06{\scriptstyle \pm0.09}$ & $99.89{\scriptstyle \pm0.08}$ & $99.97{\scriptstyle \pm0.02}$ & $99.97{\scriptstyle \pm0.01}$ \\
        D3 & \textbf{[R2] Only Round-2} & $93.79{\scriptstyle \pm0.28}$ & $97.88{\scriptstyle \pm0.18}$ & $99.38{\scriptstyle \pm0.12}$ & $99.89{\scriptstyle \pm0.05}$ & $100.00{\scriptstyle \pm0.00}$ & $100.00{\scriptstyle \pm0.00}$ \\
        \midrule
        \S~\ref{app:qualitative-comp} & \textbf{Non-linear \method-2 } & $93.68{\scriptstyle \pm0.50}$ & $96.73{\scriptstyle \pm0.23}$ & $98.55{\scriptstyle \pm0.06}$ & $99.74{\scriptstyle \pm0.05}$ & $99.96{\scriptstyle \pm0.04}$ & $99.93{\scriptstyle \pm0.03}$ \\
        \bottomrule
	\end{tabular}
}
\end{table}
