# Supplementary material for: On the Impact of Feature Heterophily on Link Prediction with Graph Neural Networks
Source: arXiv:2409.17475 source file (2024-09-26)
Supplement: Supplementary file 4 [file 096appendix-real.tex]

\clearpage
\section{Real Datasets: Details}
\label{app:real}

% \subsection{Data Description \& Limitations}

\paragraph{Datasets}  In our experiments, we use the following real-world datasets with varying levels of homophily ratios $h$. Some network statistics are given in Table~\ref{tab:5-real-results}.
\begin{itemize}
\item \textbf{Texas, Wisconsin and Cornell} are graphs representing links between web pages of the corresponding universities, originally collected by the CMU WebKB project. We used the preprocessed version  in \cite{Pei2020Geom-GCN}. In these networks, nodes are web pages, which are classified into 5 categories: course, faculty, student, project, staff. 
\item \textbf{Squirrel and Chameleon} are subgraphs of web pages in Wikipedia discussing the corresponding topics, collected by \cite{rozemberczki2019multiscale}. For the classification task, we utilize the class labels generated by \cite{Pei2020Geom-GCN}, where the nodes are categorized into 5 classes based on the amount of their average traffic.  
\item \textbf{Actor} is a graph representing actor co-occurrence in Wikipedia pages, processed by \cite{Pei2020Geom-GCN} based on the film-director-actor-writer network in \cite{tang2009social-fc}. We also use the class labels generated by \cite{Pei2020Geom-GCN}. % for this dataset. % \jiong{Actually I am not sure what they are classifying here. From \cite{Pei2020Geom-GCN} ``We classify the nodes into five categories in term of words of actor’s Wikipedia.'', which is vague.} 
\item \textbf{Cora, Pubmed and Citeseer} are citation graphs originally introduced in \cite{sen2008collective, namata2012query}, which are among the most widely used benchmarks for semi-supervised node classification \cite{shchur2018pitfalls, hu2020ogb}. Each node is assigned a class label based on the research field.
These datasets use a bag of words representation as the feature vector for each node.
\item \textbf{Cora Full} is an extended version of Cora, introduced in \cite{bojchevski2018deep, shchur2018pitfalls}, which contain more papers and research fields than Cora. This dataset also uses a bag of words representation as the feature vector for each node. 
\end{itemize}

\paragraph{Data Limitations} As discussed in \cite{shchur2018pitfalls, hu2020ogb}, Cora, Pubmed and Citeseer are widely adopted as benchmarks for semi-supervised node classification tasks; however, all these benchmark graphs display strong homophily, with edge homophily ratio $h \geq 0.7$. As a result, the wide adaptation of these benchmarks have masked the limitations of the homophily assumption in many existing GNN models. 
Open Graph Benchmark is a recent effort of proposing more challenging, realistic benchmarks with improved data quality comparing to the existing benchmarks \cite{hu2020ogb}. However, with respect to homophily, we found that the proposed OGB datasets display homophily $h > 0.5$. 

In our synthetic experiments (\S~\ref{app:synthetic}), we used \texttt{ogbn-products} from this effort to generate higher quality synthetic benchmarks while varying the homophily ratio $h$. 
In our experiments on real datasets, we go beyond the typically-used benchmarks (Cora, Pubmed, Citeseer) and consider benchmarks with strong heterophily (Table~\ref{tab:5-real-results}). That said, these datasets also have limitations, including relatively small sizes (e.g., WebKB benchmarks), artificial classes (e.g., Squirrel and Chameleon have class labels based on ranking of page traffic), or unusual network structure (e.g., \texttt{Squirrel} and \texttt{Chameleon} are dense, with many nodes sharing the same neighbors --- cf. \S~\ref{sec:real-eval}). 
We hope that this paper will encourage future work on more diverse datasets with different levels of homophily, and lead to higher quality datasets for benchmarking GNN models in the heterophily settings.
